# Supplementary material for: Dynamic correlations in the highly dilute 2D electron liquid: loss function, critical wave vector and analytic plasmon dispersion
Source: arXiv:1712.01667 source file (2017-12-05)
Supplement: Supplementary file 1 [file suppl.pdf]

Supplementary Material to:

# Dynamic correlations in the highly dilute 2D electron liquid: loss function, critical wave vector and analytic plasmon dispersion

Jürgen T. Drachta, Dominik Kreil, Raphael Hobbiger, and Helga M. Böhm
*Institut für Theoretische Physik, Johannes Kepler University, 4040 Linz, Austria*

Here, equation references without the prefix 'S' refer to the equation numbers in the main text.

## Supporting information about the fit for ultra-high densities

For a fit over a large density range it is convenient to use reduced units determined from the critical wave vector $q_c$ for Landau damping. Wave verctors are expressed as $\underline{q} = \bar{q}/\bar{q}_c$ and frequencies are then expressed in the critical frequency $\omega_c \equiv \omega_{pl}(q_c)$, easily found from the upper single particle band edge as $\hbar(q_c^2 + 2q_c k_F)/2m^*$. The following approximation for the turned out to describe the plasmon dispersion excellently

$$\underline{\omega}_{pl}^{fit}(q, r_s) \equiv \frac{\omega_{pl}^{fit}(q, r_s)}{\omega_{pl}(q_c, r_s)} = \sqrt{\underline{q}}\, P_{[2,4]}(\underline{q}, r_s)\ , \tag{S.1}$$

which can be expanded to

$$\underline{\omega}_{pl}^{fit} = \sqrt{\underline{q}}\, \frac{p_0 + p_1\, \underline{q} + p_2\, \underline{q}^2}{1 + \tilde{p}_1\, \underline{q} + \tilde{p}_2\, \underline{q}^2 + \tilde{p}_3\, \underline{q}^3 + \tilde{p}_4\, \underline{q}^4} \tag{S.2}$$

Next, these coefficients were fitted in a sectioned step to the density parameter $r_s$ via the ansatz:

$$p_i = \pm c_0^{(i)} \pm c_1^{(i)}\, r_s \pm \left(c_{3/2}^{(i)}\, r_s\right)^{3/2} \pm \left(c_2^{(i)}\, r_s\right)^2 \tag{S.3a}$$

$$\tilde{p}_i = \pm \tilde{c}_0^{(i)} \pm \tilde{c}_1^{(i)}\, r_s \pm \left(\tilde{c}_{3/2}^{(i)}\, r_s\right)^{3/2} \pm \left(\tilde{c}_2^{(i)}\, r_s\right)^2 \tag{S.3b}$$

The coefficients can be nailed down according to the limits in Eq. (D.1) and Eq. (D.2) that were calculated as a first step. Using the expression (25) found for $q_c(r_s)$, this procedure gives the following relations for the coefficients up to $\mathcal{O}(q^1)$

$$p_0 = 2^{3/4}\sqrt{r_s}\, \frac{\sqrt{q_c/k_F}}{\hbar\omega_c/\varepsilon_F} = \frac{2^{3/2}}{r_s}\, \frac{\sqrt{q_c a_B^*}}{\hbar\omega_c[\mathrm{Ry}^*]} \tag{S.4}$$

$$p_1 - p_0\, \tilde{p}_1 = \frac{1 + n\kappa(r_s)\varepsilon_F}{2^{7/4}\sqrt{r_s}}\, \frac{(q_c/k_F)^{3/2}}{\hbar\omega_c/\varepsilon_F} = \frac{1 + \kappa(r_s)/\kappa^0(r_s)}{2^{3/2}\, r_s}\, \frac{(q_c a_{B^*})^{3/2}}{\hbar\omega_c[\mathrm{Ry}^*]}\ . \tag{S.5}$$

Here, the non-interacting compressibility in 2D is $\kappa^0 = 1/n\varepsilon_F$. The values of the remaining parameters $p_i\,, \tilde{p}_j$ were computed numerically.

To achieve the best results, a final fitting loop incorporating aspects of generic algorithms (e.g. mutation and crossover) was applied. As objective function, a weighted least-square-error was used. This resulted in the coefficients given in Tables D.2 and S.1. In figure 3, the final approximant is compared to the numerical data with the former values; the parameters of table S.1 are superior when $r_s \gtrsim 30$ and correct within $5\%$ down to $r_s \gtrsim 10$. Note that conversion from reduced to real units introduces a density dependent scaling, as $\varepsilon_F \propto r_s^{-2}$, having a strong impact for dense systems. As there the RPA gives results of sufficient accuracy, the fit proposed here is designed to capture the wide density range of intermediate $r_s$ up the predicted Wigner crystallization.

| | $c_0$ | $c_1$ | $c_{3/2}$ | $c_2$ |
|---|---|---|---|---|
| $p_1$ | (−) 0.823609 | (−) 0.187093 | (+) 0.0939417 | (−) 0.0363816 |
| $p_2$ | (+) 0.0869994 | (+) 0.162949 | (−) 0.107642 | (+) 0.0471211 |
| $\tilde{p}_1$ | (−) 1.4253 | (+) 0.0344364 | (−)0.0403881 | (+) 0.0271882 |
| $\tilde{p}_2$ | (+) 0.505042 | (−)0.046883 | (+) 0.0667535 | (−)0.0166585 |
| $\tilde{p}_3$ | (−) 0.485973 | (+) 0.210121 | (−)0.16216 | (+) 0.0588428 |
| $\tilde{p}_4$ | (+) 0.288709 | (−)0.112816 | (+) 0.104454 | (−)0.0454723 |

**Table S.1.** Meta–Parameters as well as the used signs for the plasmon fit given in Eq.(S.2)

## Supporting information about the width of the plasmon mode

The lifetime of the plasmon, proportional to the inverse FWHM of the peak in $-\mathrm{Im}\,\chi(q,\omega)$, clearly depends on the plasmon's wavelength. For the Lorentzian in Eq. (27) of the main text we found

$$\Gamma^{\mathrm{fit}}_{\mathrm{2p2h}} = \underline{q}^{7/2}\left(p^{\Gamma}_{0} + p^{\Gamma}_{1/2}\,\underline{q}^{1/2} + p^{\Gamma}_{3/2}\,\underline{q}^{3/2} + p^{\Gamma}_{4/2}\,\underline{q}^{4/2}\right), \quad \underline{q} = q/q_{\mathrm{c}} \tag{S.6a}$$

$$p^{\Gamma}_{i/2}(r_{\mathrm{s}}) = c^{\Gamma}_{i/2,0} + c^{\Gamma}_{i/2,1}\,r_{\mathrm{s}} + c^{\Gamma}_{i/2,2}\,r_{\mathrm{s}}^2\,, \tag{S.6b}$$

with the coefficients given in table S.2.

These coefficients were obtained by fitting the actual 2p2h peak to a Lorentzian. Alternatively, one can start with the expression for $\chi^{\mathrm{2p2h}}(q,\omega)$ given in the main text in Eqs. (16)-(22). Written as a single numerator $N(q,\omega)$ and denominator $D(q,\omega)$ this is then Taylor expanded around $\omega_{\mathrm{pl}}(q)$

$$-\,\mathrm{Im}\,\chi^{\mathrm{2p2h}}(q,\omega) \;=\; -\mathrm{Im}\,\frac{N(q,\omega)}{D(q,\omega)} \;\approx\; \frac{\mathrm{Re}N(q,\omega)\,\mathrm{Im}D(q,\omega)/c(q)^2}{\left(\omega_{\mathrm{pl}}(q)-\omega\right)^2 + \left(\mathrm{Im}D(q,\omega)/c(q)\right)^2}\,, \tag{S.7}$$

where $c(q) \equiv \partial \mathrm{Re}N/\partial\omega|_{\omega_{\mathrm{pl}}}$ and $\mathrm{Im}N\,\mathrm{Re}D \ll \mathrm{Re}N\,\mathrm{Im}D$. All functions contributing to $N$ and $D$ being available in the full implementation of $\chi^{\mathrm{2p2h}}$, we confirmed that the Lorentzian (S.7) (blue full curve in Fig. 4) closely matches that obtained with (S.6) (green dotted curve).

| $p^{\Gamma}_{i}(r_{\mathrm{s}})$ | $c^{\Gamma}_{i/2,0}$ | $c^{\Gamma}_{i/2,1}$ | $c^{\Gamma}_{i/2,2}$ |
|---|---|---|---|
| $p^{\Gamma}_{0}(r_{\mathrm{s}})$ | 40.0298 | -6.9251 | 0.315122 |
| $p^{\Gamma}_{1/2}(r_{\mathrm{s}})$ | -94.6375 | 16.0834 | -0.681113 |
| $p^{\Gamma}_{3/2}(r_{\mathrm{s}})$ | 129.301 | -21.1785 | 0.803636 |
| $p^{\Gamma}_{4/2}(r_{\mathrm{s}})$ | -74.6926 | 12.0368 | -0.437983 |

**Table S.2.** Coefficients for the fit of the dispersion of the sheet plasmon used in (S.6).

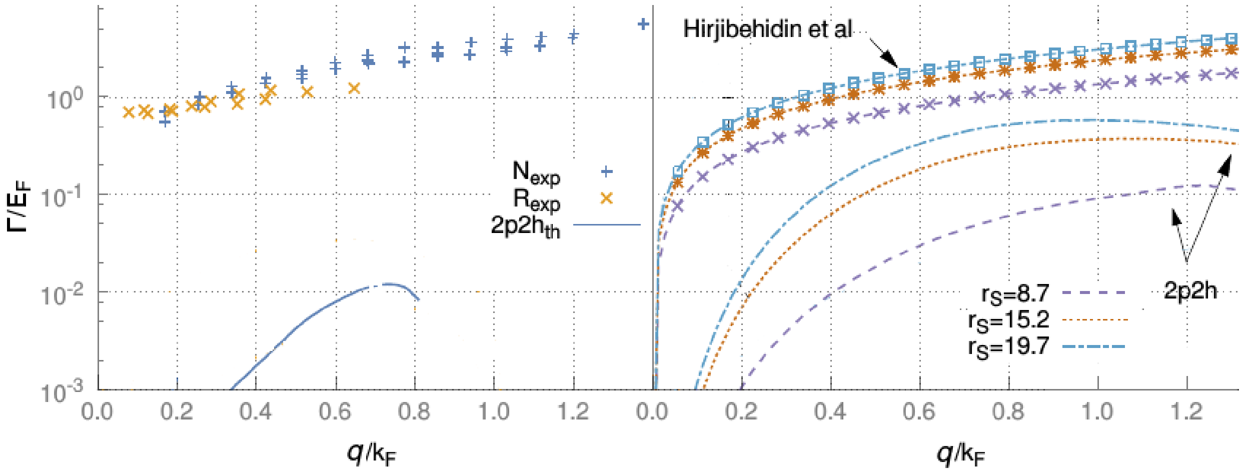


**Figure S.1.** Plasmon half-width $\Gamma$ due to 2–pair excitations (lines) compared with measured values (symbols). Left: dense case (Nagao et al. [17], $r_S = 1.2$ and Rugeramigabo et al. [18], $r_S = 1.0$). Right: highly dilute case (Hirjibehedin et al. [19, 20], $r_S \approx 9 \ldots 20$). In units of Fermi energies and wavevectors, higher lying curves correspond to higher $r_S$.

In Fig. S.1 we give the comparison with actually measured half widths $\Gamma$, proportional to a plasmon's life time $\tau^{-1}$. As also the case in the bulk, plasmon decay into multi–pair excitations is not possible at $q=0$ and experimental $\Gamma(0)$ are due to other mechanisms. For dense 2DEGs, where multi-pair excitations get neglishible, plasmon losses by pair excitations are more than 2 orders of magnitude below the measured data. For the ultra-dilute samples the 2p2h damping is still an order of magnitude too low.

Certainly, not only the magnitude, but also the overall shape of the 2p2h width-dispersion does not satisfactorily match the experimental data. The decrease of $\Gamma(q)$ when it approaches the single–particle band is expected to to be overcome by higher order multi-pair effects which get relevant with increasing $q$ and $r_S$.

# for our eyes only

## Factors for rescaling

Useful expressions, needed so often, that we want to have them at hand:

material propts.: eff. charge $e^{*2} \equiv e^2/\varepsilon_{\rm b}$, density propts.: $k_{\rm F}^2 = 2\pi n$, mean radius: area $\mathcal{F} \equiv N\,(a^2\pi) \to a^2 = 1/n\pi$

$$\begin{aligned} a_{\rm B}^* &\equiv \frac{\hbar^2}{m^*\,e^{*2}} = \frac{m_0}{m^*}\varepsilon_{\rm b}\,a_{\rm B}\,, \quad a_{\rm B} = 0.529177\,\text{Å} \\ {\rm Ry}^* &\equiv \frac{e^{*2}}{2a_{\rm B}^*} = \frac{m^*}{m_0}\frac{1}{\varepsilon_{\rm b}^2}\,{\rm Ry}\,, \quad {\rm Ry} = 13.6057\,{\rm eV} \end{aligned} \;;\quad \begin{aligned} \frac{q}{k_{\rm F}} &= q a_{\rm B}^* \frac{r_{\rm S}}{\sqrt{2}} = qa\frac{1}{\sqrt{2}} \\ \frac{\hbar\omega}{E_{\rm F}} &= \frac{\hbar\omega}{{\rm Ry}^*}\frac{r_{\rm S}^2}{2} \end{aligned} \;;\quad a = a_{\rm B}^* r_{\rm S} = \frac{\sqrt{2}}{k_{\rm F}}\;;$$

Material parameters of the GaAs-AlGaAs QWell:
(from ioffe.ru/…/GaAs/basic, ioffe.ru/…/AlGaAs/basic @300 K (1); and from ecee/…/effmass.htm )

$$\begin{aligned} \varepsilon_{\rm b}^{\rm GaAs} &= 12.9 \\ \left(\tfrac{m^*}{m_0}\right)_e^{\rm GaAs} &= 0.063\ (1) \quad 0.067\ (2) \\ \left(\tfrac{m^*}{m_0}\right)_{\rm hh}^{\rm GaAs} &= 0.51\ \ (1) \quad 0.45\ \ (2) \\ \left(\tfrac{m^*}{m_0}\right)_{\rm lh}^{\rm GaAs} &= 0.082\ (1) \quad 0.082\ (2) \end{aligned} \;;\quad \begin{aligned} \varepsilon_{\rm b}^{{\rm Al}_x{\rm Ga}_{1-x}{\rm As}} &= 12.90 - 2.84\,x \\ \left(\tfrac{m^*}{m_0}\right)_e^{{\rm Al}_x{\rm Ga}_{1-x}{\rm As}} &= 0.063 + 0.083\,x\ (x < 0.45) \\ \left(\tfrac{m^*}{m_0}\right)_{\rm hh}^{{\rm Al}_x{\rm Ga}_{1-x}{\rm As}} &= 0.51 + 0.25\,x \\ \left(\tfrac{m^*}{m_0}\right)_{\rm lh}^{{\rm Al}_x{\rm Ga}_{1-x}{\rm As}} &= 0.082 + 0.068\,x \end{aligned}$$

Hirjibehedin et al. use $\varepsilon_{\rm b} = 13$ and $m^* = 0.67\,m_0$, therefore

$$a_{\rm B}^* = 194\,a_{\rm B} = 102.68\,\text{Å} \approx 10^{-6}\,{\rm cm}\,; \quad {\rm Ry}^* = 3.9645\,10^{-4}\,{\rm Ry} = 5.394\,{\rm meV}$$

their well width is

$$L = 330\text{Å} \;\Rightarrow\; L \approx 33\,a_{\rm B}^*$$

(lattice const: $a_{\rm latt}^{\rm GaAs} = 5.65325\,\text{Å}$, $a_{\rm latt}^{\rm AlGaAs} = 5.6533 + 0.0078x\,\text{Å}$, thus $L \approx 60 a_{\rm latt}$)

free & full compressibility:

$$\frac{1}{n\kappa_{\rm 2D}^0} = 1\varepsilon_{\rm F}\;; \quad \frac{\kappa^0}{\kappa} = 1 - \frac{\sqrt{2}}{\pi}r_{\rm S} - \frac{r_{\rm S}^3}{8}\left(\frac{\varepsilon'(r_{\rm S})}{{\rm Ry}^*} - r_{\rm S}\frac{\varepsilon''(r_{\rm S})}{{\rm Ry}^*}\right)$$

## Plasmon dispersion and limits ($L = 0$)

The numerically calculated plasmon exhibits the following asymptotic behaviour

$$\lim_{q\to 0} \bar\omega_{\rm pl}(\bar q) = a_{1/2}\sqrt{\bar q} + a_{3/2}\,\bar q^{3/2} + a_{5/2}\,q^{5/2} \tag{S.8}$$

with $a_{1/2} = 2^{3/4}\sqrt{r_{\rm S}}$; $a_{3/2}$ is known from the compressibility but was also determined by fitting the numerical 2p2h data. 'This corresponds extremely well to the coefficients obtained directly from Eq.()'. ▶ hmb: wich Eq.? check Jürgen's thesis on that.◀ We find

$$a_{3/2} = -0.09738 r_{\rm s} + 0.0010275 r_{\rm s}^2 - \frac{0.36762}{\sqrt{r_{\rm s}}} + \frac{0.96752}{r_{\rm s}}, \tag{S.9}$$

$$a_{5/2} = -0.609032 + 0.0793028\,r_{\rm s} - 0.00810535\,r_{\rm s}^2\,. \tag{S.10}$$

In the vicinity of $q_{\rm c}$, where $\underline{q} \approx 1$, the plasmon dispersion can be modelled as

$$\lim_{\bar q\to 1} \bar\omega_{\rm pl}(\bar q) \approx \bar\omega_{\rm c} + a_{\rm c1}\,\bar q + a_{\rm c2}\,\bar q^2 + a_{\rm c3}\,\bar q^3 \tag{S.11}$$

in a good agreement with the numerical data with the following coefficients:

$$a_{c1} = 0.457594 + 1.05355\sqrt{r_s} - 0.0485302\, r_s \quad (S.12)$$
$$a_{c2} = 0.500685 - 1.82524\sqrt{r_s} + 0.0591981\, r_s \quad (S.13)$$
$$a_{c3} = 0.0417223 + 0.771698\sqrt{r_s} - 0.0106679\, r_s \quad (S.14)$$

### Splitting into different contributions, see Chapter 5

Hirjibehedin et al. [19, 20] published the plasmon dispersion in the form (=their best fit)

$$\omega_{pl} = \omega_0\sqrt{1+\xi\, q}$$

where they split the length $\xi$ into the following terms:

**nonlocal:** $\xi_{nl} > 0$ is the analytic contribution from RPA. It is constant (i.e. $r_S$−independent) in 'real' (e.g. $a_B^*$) units (hmb: one of the peculiarities of the 2DEG, like $q_{TF} = 2/a_B^*$)

**width:** $-|\xi_L| < 0$ is the finite thickness effect, also not effected by the density (in real units)

**correlation:** $-|\xi_{cor}| < 0$ contains all correlations *beyond* the RPA (=nonlocal). This length depends on the density (as correlations should!). In units of $a = a_B^* r_S$ Hirjibehedin+ find it more or less constant, rephrased: $-|\xi_{cor}| \propto r_S^1$

**temperature:** $\xi_T > 0$, is the effect due to measuring at finite $T \gtrsim 1$K (there is a single 0.25K sample ($r_S = 15$), the next lowest $T \approx 1.8$K). This term, again, is found to be linear in $r_S$ if given in real units

### Experimental determination of $\xi_{corr}$

In Fig.4 of their work, Hirji. fitted the total $\xi$ of several samples. They claim that the nonlocal and the thickness effect cancel each other, therefore only temperature as well as correlation parts remain. This $\xi = \xi_{cor} + \xi_T$ is shown in Fig.4 for all samples and several temperatures. Extrapolation to $T \to 0$ implies that there only the correlation part remains.

### @ bare RPA with form factor

appendix E, Eqs.(E2-3) (eq: Fqtoo), (eq: wpl_LRPA qtoo), 1 order further in $q$:

$$F(q\to 0) = 1 - q\,\xi^L_{width} + (q\Delta z)^2 + f_3\, q^3\,,$$

$$\frac{\omega^L_{pl}(q)}{\omega_0(q)} \approx 1 + q^2\left(\frac{a_B^{*2}}{32} + \frac{\Delta z^2}{2}\right) + q^3\left(\frac{a_B^{*3}(1+4r_S^2)}{64} + \frac{f_3}{2}\right).$$

This $q^3$ term is where the first $r_S$−dependence comes in.

btw, our smallest $\omega^{2p2h}_{pl}(q)$ is always far below the $\sqrt{q}$; rephrased: the corrs will always pull down the larger $q$ more than $q\to 0$. ie, we won't easily get a $\sqrt{}$−like form as in the expt. — es sei denn, es kommt wieder $L$ zu hilfe, weil $e^{-qz}$ ja bei kleinen $q$ wirkt.

a brief note on $q_c(r_s)$:
For $L = 0$ and the bare Coulomb potential Eq. (24) can be written as

$$1 + \frac{q_c a_B^*}{2} = \sqrt{1 + \frac{\sqrt{2}}{r_S}\,\frac{1}{q_c a_B^*}} \quad \Longleftrightarrow \quad (q_c a_B^*)^3 + 4(q_c a_B^*)^2 = \frac{4\sqrt{2}}{r_S} \quad (S.15)$$

This implies $q_c(r_S \to 0)$ diverges $\propto r_S^{-1/3}$ in real units ► hmb: whatever this may mean◄

## Some text-phrases

Plasmons of charged bosons interacting via a Yukawa potential were investigated in this formalism in [25]

Dom: One has to note here, that Eq. (??) is not fulfilled exactly by the fit given in Eq. (S.2). A small deviation was allowed for easy relaxation of the fitting result. ► hmb: keep this or moveto 4us?◄

## Unfinished: Collective approximation for the Neilson formula

Comparison with Neilson [42]:

$$\chi^{0\gamma}_{\mathrm{PPA}} = \frac{q^2/m}{\omega\,(\omega + i\gamma^{\mathrm{s}})} \tag{S.16}$$

► hmb: intermediate result:◄

$$\chi^{\mathrm{NSSS}}_{\mathrm{PPA}} = \frac{\hbar^2 q^2/m}{\hbar^2\omega\,(\omega + i\gamma^{\mathrm{s}}) - \left[2t\,V_{\mathrm{ph}} - \hbar^2(\gamma - \gamma^{\mathrm{s}})\right]} \tag{S.17}$$

looks like an $i$ is missing in the NSSS formula

## Some Eqs from our fist version, in Fermi units

Indicating reduced wave vectors $\bar{q} = q/k_{\mathrm{F}}$ and energies $\hbar\bar{\omega} = \hbar\omega/\epsilon_{\mathrm{F}}$ via a bar:

borders of the single particle-hole band: $\bar{\omega}_{\mathrm{ph}} = \bar{q}^2 \pm 2\bar{q}$

► hmb: im main dzt dimbehaftet◄ high density (= bare RPA), long wavelength plasmon dispersion:

$$\lim_{\bar{q}\to 0} \bar{\omega}^{\mathrm{RPA}}_{\mathrm{pl}}(\bar{q}) = \bar{\omega}_0 \left[1 + \frac{3}{4\sqrt{2}\,r_{\mathrm{s}}}\,\bar{q} + \mathcal{O}\left(\bar{q}^2\right)\right]$$

with the classical plasmon limit $\omega_0 = 2^{3/4}\sqrt{r_{\mathrm{s}}}\,\bar{q}$ and in GRPA = Eq.14 = (eq: kappa_SR omp) of the main text

$$\lim_{\bar{q}\to 0} \bar{\omega}^{\mathrm{GRPA}}_{\mathrm{pl}}(\bar{q}) = \bar{\omega}_0 \left[1 + \frac{1 + 2\bar{\kappa}(r_{\mathrm{s}})}{2^{5/2}\,r_{\mathrm{s}}}\,\bar{q} + \mathcal{O}\left(\bar{q}^2\right)\right]$$

# References


[1] R. Wood, Remarkable optical properties of the alkali metals, Physical Review 44 (1933) 353.

[2] W. Lang, Geschwindigkeitsverluste mittelschneller Elektronen beim Durchgang durch dünne Metallfolien, Optik 3 (1948) 233–246.

[3] G. Ruthemann, Diskrete Energieverluste mittelschneller Elektronen beim Durchgang durch dünne Folien, Annalen der Physik 437 (1948) 113–134.

[4] D. Bohm, D. Pines, A collective description of electron interactions: III. Coulomb interactions in a degenerate electron gas, Physical Review 92 (1953) 609.

[5] S. Allen Jr, D. Tsui, R. Logan, Observation of the two-dimensional plasmon in silicon inversion layers, Physical Review Letters 38 (1977) 980.

[6] N. Armbrust, J. Güdde, U. Höfer, S. Kossler, P. Feulner, Spectroscopy and Dynamics of a Two-Dimensional Electron Gas on Ultrathin Helium Films on Cu(111), Physical Review Letters 116 (2016) 256801.

[7] S. D. Sarma, Q. Li, Intrinsic plasmons in two-dimensional Dirac materials, Physical Review B 87 (23) (2013) 235418.

[8] S. Ta Ho, H. Anh Le, T. Le, D. Chien Nguyen, V. Nam Do, Effects of temperature, doping and anisotropy of energy surfaces on behaviors of plasmons in graphene, Physica E 58 (2014) 101–105.

[9] D. Van Tuan, Q. N. Khanh, Plasmon modes of double-layer graphene at finite temperature, Physica E 54 (2013) 267–272.

[10] J. Hofmann, S. Das Sarma, Plasmon signature in Dirac-Weyl liquids, Physical Review B 91 (2015) 241108.

[11] A. Thakur, R. Sachdeva, A. Agarwal, Dynamical polarizability, screening and plasmons in one, two and three dimensional massive Dirac systems, Journal of Physics: Condensed Matter 29 (2017) 105701.

[12] I. Grosu, L. Tugulan, Plasmon dispersion in quasi-one- and one-dimensional systems with non-magnetic impurities, Physica E 40 (3) (2008) 474–477.

[13] G. Giuliani, G. Vignale, Quantum theory of the electron liquid, Cambridge University Press, 2005.

[14] Ž. B. Lošić, Spectral function of the two-dimensional system of massless Dirac electrons, Physica E 58 (2014) 138–145.

[15] D. Vigil-Fowler, S. G. Louie, J. Lischner, Dispersion and line shape of plasmon satellites in one, two, and three dimensions, Physical Review B 93 (2016) 235446.

[16] M. Polini, R. Asgari, G. Borghi, Y. Barlas, T. Pereg-Barnea, A. H. MacDonald, Plasmons and the spectral function of graphene, Physical Review B 77 (2008) 081411.

[17] T. Nagao, T. Hildebrandt, M. Henzler, S. Hasegawa, Dispersion and Damping of a Two-Dimensional Plasmon in a Metallic Surface-State Band, Physical Review Letters 86 (2001) 5747–5750.

[18] E. P. Rugeramigabo, T. Nagao, H. Pfnür, Experimental investigation of two-dimensional plasmons in a $DySi_2$ monolayer on Si(111), Phys. Rev. B 78 (2008) 155402.

[19] C. F. Hirjibehedin, A. Pinczuk, B. S. Dennis, L. N. Pfeiffer, K. W. West, Evidence of electron correlations in plasmon dispersions of ultralow density two-dimensional electron systems, Physical Review B 65 (2002) 161309.

[20] M. Eriksson, A. Pinczuk, B. Dennis, C. Hirjibehedin, S. Simon, L. Pfeiffer, K. West, Collective excitations in low-density 2D electron systems, Physica E 6 (1) (2000) 165–168.

[21] X. Hao, Z. Wang, M. Schmid, U. Diebold, C. Franchini, Coexistence of trapped and free excess electrons in $\mathrm{SrTiO_3}$, Physical Review B 91 (2015) 085204.

[22] A. Faridi, R. Asgari, Plasmons at the $LaAlO_3/SrTiO_3$ interface and in the graphene-$LaAlO_3/SrTiO_3$ double layer, Physical Review B 95 (2017) 165419.

[23] H. M. Böhm, R. Holler, E. Krotscheck, M. Panholzer, Dynamic many-body theory: Dynamics of strongly correlated Fermi fluids, Physical Review B 82 (2010) 224505.

[24] C. E. Campbell, E. Krotscheck, T. Lichtenegger, Dynamic many-body theory: Multiparticle fluctuations and the dynamic structure of $^4\mathrm{He}$, Physical Review B 91 (2015) 184510.

[25] J. Halinen, V. Apaja, M. Saarela, Effect of external screening on plasmons, Physica E 18 (1) (2003) 346–347.

[26] E. H. Hwang, S. Das Sarma, Plasmon dispersion in dilute two-dimensional electron systems: quantum–classical and Wigner crystal – electron liquid crossover, Physical Review B 64 (2001) 165409.

[27] B. Davoudi, M. Polini, G. F. Giuliani, M. P. Tosi, Analytical expressions for the charge-charge local-field factor and the exchange-correlation kernel of a two-dimensional electron gas, Physical Review B 64 (2001) 153101.

[28] P. Gori-Giorgi, S. Moroni, G. B. Bachelet, Pair-distribution functions of the two-dimensional electron gas, Physical Review B 70 (2004) 115102.

[29] M. Polini, M. Tosi, Many-body physics in condensed matter systems (Publications of the Scuola Normale Superiore) (v.4), Edizioni della Normale, ISBN 9788876421921, 2006.

[30] S. Moroni, D. M. Ceperley, G. Senatore, Static response from quantum Monte Carlo calculations, Physical Review Letters 69 (1992) 1837–1840.

[31] A. Fabrocini, S. Fantoni, E. Krotscheck, Introduction to Modern Methods of Quantum Many–Body Theory and their Applications, vol. 7 of *Advances in Quantum Many–Body Theory*, World Scientific, Singapore, 2002.

[32] D. Kreil, R. Hobbiger, J. T. Drachta, H. M. Böhm, Excitations in a spin-polarized two-dimensional electron gas, Physical Review B 92 (2015) 205426.

[33] G. Senatore, S. Moroni, D. M. Ceperly, The local field of the electron gas, in: W. D. W. D. Kraeft, M. Schlanges

(Eds.), Proceedings of the (Binz Germany) International Conference on the Physics of Strongly Coupled Plasmas, World Scientific, Singapore, 429–434, 1996.

[34] G. Niklasson, Dielectric function of the uniform electron gas for large frequencies or wave vectors, Physical Review B 10 (1974) 3052–3061.

[35] N. Bhukal, Priya, R. Moudgil, Dispersion of two-dimensional plasmons in GaAs quantum well and Ag monolayer, Physica E 69 (2015) 13–18.

[36] K. Aharonyan, Dielectric function and collective plasmon modes of a quasi-two-dimensional finite confining potential semiconductor quantum well, Physica E 43 (9) (2011) 1618–1624.

[37] N. Iwamoto, Sum rules and static local-field corrections of electron liquids in two and three dimensions, Physical Review A 30 (1984) 3289–3304.

[38] N. D. Mermin, Lindhard Dielectric Function in the Relaxation-Time Approximation, Physical Review B 1 (1970) 2362–2363.

[39] A. Holas, S. Rahman, Dynamic local-field factor of an electron liquid in the quantum versions of the Singwi-Tosi-Land-Sjölander and Vashishta-Singwi theories, Phys. Rev. B 35 (1987) 2720–2731.

[40] A. Yurtsever, V. Moldoveanu, B. Tanatar, Dynamic correlation effects on the plasmon dispersion in a two-dimensional electron gas, Physical Review B 67 (2003) 115308.

[41] M. Tas, B. Tanatar, Plasmonic contribution to the van der Waals energy in strongly interacting bilayers, Physical Review B 81 (2010) 115326.

[42] D. Neilson, L. Świerkowski, A. Sjölander, J. Szymański, Dynamical theory for strongly correlated two-dimensional electron systems, Physical Review B 44 (1991) 6291–6305.

[43] R. Hobbiger, J. T. Drachta, D. Kreil, H. M. Böhm, Phenomenological plasmon broadening and relation to the dispersion, Solid State Communications 252 (2017) 54 – 58.

[44] K. Sturm, Electron energy loss in simple metals and semiconductors, Advances in Physics 31 (1982) 1–64.

[45] T. Fukuda, N. Hiraiwa, T. Mitani, T. Toyoda, Plasmon dispersion of a two-dimensional electron system with finite layer width, Physical Review B 76 (2007) 033416.

[46] H. Godfrin, M. Meschke, H.-J. Lauter, A. Sultan, H. M. Böhm, E. Krotscheck, M. Panholzer, Observation of a roton collective mode in a two-dimensional Fermi liquid, Nature 483 (2012) 576–579.

[47] A. Agarwal, M. Polini, G. Vignale, M. E. Flatté, Long-lived spin plasmons in a spin-polarized two-dimensional electron gas, Physical Review B 90 (15) (2014) 155409.

[48] R. Asgari, B. Davoudi, M. Polini, G. F. Giuliani, M. P. Tosi, G. Vignale, Quasiparticle self-energy and many-body effective mass enhancement in a two-dimensional electron liquid, Physical Review B 71 (2005) 045323.

[49] R. Asgari, T. Gokmen, B. Tanatar, M. Padmanabhan, M. Shayegan, Effective mass suppression in a ferromagnetic two-dimensional electron liquid, Physical Review B 79 (2009) 235324.

[50] E. Krotscheck, J. Springer, Physical Mechanisms for Effective Mass Enhancement in 3He, Journal of Low Temperature Physics 132 (5) (2003) 281–295.

[51] E. Feenberg, Theory of quantum fluids, Pure and applied physics, Academic Press, ISBN 9780122508509, 1969.

[52] C. C. Chang, C. E. Campbell, Density dependence of the roton spectrum in liquid $^4\mathrm{He}$, Physical Review B 13 (1976) 3779–3782.

[53] Y. Wang, E. W. Plummer, K. Kempa, Foundations of Plasmonics, Advances in Physics 60 (5) (2011) 799–898.
